# Supplementary material for: Anomalous momentum diffusion in a dissipative many-body system
Source: arXiv:1905.04808 ancillary file (2019-05-12)
Supplement: Supplementary file 1 [file AnomalousDiffusion_SM_arxiv_v1.pdf]

# Supplementary Information for: Anomalous momentum diffusion in a dissipative many-body system

Raphaël Bouganne,[1] Manel Bosch Aguilera,[1] Alexis Ghermaoui,[1] Jérôme Beugnon,[1] and Fabrice Gerbier[1]

[1] *Laboratoire Kastler Brossel, Collège de France, ENS-PSL Research University, Sorbonne Université, CNRS, 11 place Marcelin-Berthelot, 75005 Paris.*

(Dated: May 3, 2019)

## CONTENTS


Supplementary text 1

I. Experimental details 1
- A. Preparation of two-dimensional quantum gases in optical lattices 1
- B. Calibration of the spontaneous emission rate 1
- C. Image processing 2

II. Theoretical background 2
- A. Band structure and notations 2
- B. Bose-Hubbard model 2
- C. Theoretical description of light scattering 2
- D. Non-interacting atoms: quasi-momentum diffusion and inter-band transitions 3
- E. Two atoms and two wells 4

III. Analysis of a continuous measurement model 4
- A. Single-band zero-range model 4
- B. Anomalous diffusion in the algebraic regime 5
- C. Nearest-neighbor coherence 6

IV. Light-induced inelastic losses 7
- A. Scaling behavior in the loss dynamics 7
- B. Interpretation of the loss dynamics 8
- C. Estimation of the semi-classical loss rate 8

V. Extended model: External confinement and losses 8
- A. Inhomogeneous density distribution 8
- B. Including atom losses 9

VI. Analysis of the momentum distributions 10
- A. Direct analysis 10
- B. Extraction of coherence from the momentum profiles 11
- C. Evolution of condensed fraction 13
- D. Inter-band transitions 13

References 15


## SUPPLEMENTARY TEXT

## I. EXPERIMENTAL DETAILS

### A. Preparation of two-dimensional quantum gases in optical lattices

We previously described in [2] the preparation of the gas in the lowest Bloch band of the optical lattice. Briefly, starting from a Bose-Einstein condensate (BEC) in a crossed optical dipole trap with frequencies $\omega_{x,y,z} = 2\pi \times \{60, 230, 260\}\,\mathrm{Hz}$, we first ramp up a vertical lattice (VL) to its maximum depth $V_z \approx 27\,E_\mathrm{R}$. We then smoothly extinguish the crossed optical dipole trap and finally slowly increase the horizontal lattices (HL) depth to the final value $V_\perp$. This results in a stack of independent two-dimensional systems in each plane of the VL prepared in the fundamental Bloch band of the HL.

### B. Calibration of the spontaneous emission rate

The on-resonance Rabi frequency $\Omega_\mathrm{L}$ characterizing the strength of laser excitation is proportional to the square root of the laser power, $\Omega_\mathrm{L} = a\sqrt{P_\mathrm{L}}$. The coefficient $a = \Gamma_0/(w_\mathrm{L}\sqrt{\pi I_\mathrm{sat}})$ is given by the laser waist ($1/\mathrm{e}^2$ radius) $w_\mathrm{L}$, the saturation intensity $I_\mathrm{sat} \approx 0.14\,\mathrm{mW/cm^2}$ and $\Gamma_0$. We set $\Omega_\mathrm{L}$ to weakly saturate the optical transition such that the excited state population is small. The rate of spontaneous emission for a single atom in free space is well approximated by $\gamma_\mathrm{sp} \approx s\Gamma_0/2 = 520\,\mathrm{s^{-1}}$.

We observe Rabi oscillations on the intercombination transition induced by the dissipation laser, and use the measured oscillation frequency to calibrate the coefficient $a$. More precisely, we shine the dissipation laser on a BEC. For experimental convenience, we fix the pulse duration $T$ and vary the laser power $P_\mathrm{L}$. We record absorption images after a time of flight long compared to $\Gamma_0^{-1}$, so that all excited atoms have decayed back to the ground state when the image is taken. The width of the measured momentum distribution reflects the internal state of the atoms before decay due to the recoil of excited atoms when a photon is spontaneously emitted. As shown in Fig. S1A, the momentum width displays oscillations, and can be taken as a proxy of the population transferred to the excited state. We infer the oscillation period $aT$ from such curves taken at resonance ($\delta_\mathrm{L} = 0$) by fitting a sinusoidal function to the data, and

obtained $a \approx 2\pi \times 2.88\,\mathrm{MHz/mW^{1/2}}$. We independently calibrated the waist of the excitation laser using Gaussian optics propagation and found $w_\mathrm{L} \sim 1\,\mathrm{mm}$, leading to $a \approx 2\pi \times 2.76\,\mathrm{MHz/mW^{1/2}}$, in excellent agreement with the measured value.

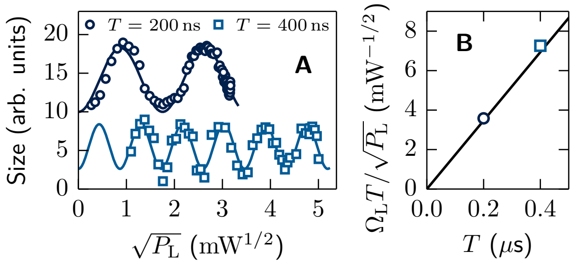


FIG. S1. **Calibration of Rabi frequency.** (**A**) Rabi oscillations on the $^1\mathrm{S}_0 - {}^3\mathrm{P}_1$ transition with chosen pulse time $T$ and varying laser power $P_\mathrm{L}$. The cloud size is normalized arbitrarily and curves are vertically shifted for clarity. (**B**) Inferred (data points) and calculated (solid line) oscillation period $aT = \Omega_\mathrm{L} T/\sqrt{P_\mathrm{L}}$.

### C. Image processing

Absorption images on the $^1\mathrm{S}_0 - {}^1\mathrm{P}_1$ transition are taken after a time-of-flight expansion of the gas of 20 ms. The probe beam propagates vertically and integrates the density distribution of the various planes. The resulting two-dimensional atomic distribution then reflects the momentum distribution of the gases before expansion [3]. The image-space to momentum-space conversion factor is $60\,\mu\mathrm{m} \equiv 2\pi/\lambda_\mathrm{lat} = k_\mathrm{lat}$. We pre-process the images before analysis to remove experimental artifacts using a *best-reference picture* algorithm described in [4].

## II. THEORETICAL BACKGROUND

### A. Band structure and notations

We consider a lattice with negligible tunneling along the vertical $z$ direction. We denote by $\boldsymbol{r}_i = (x_i, y_i)$ a lattice site position, by $w(\boldsymbol{r} - \boldsymbol{r}_i)$ the Wannier function in the fundamental Bloch band centered at $\boldsymbol{r}_i$, by $\hat{a}_i$ the corresponding annihilation operator, and by $\hat{n}_i = \hat{a}_i^\dagger \hat{a}_i$ the number operator counting the occupation of site $i$.

In a cubic lattice, energy bands are labeled by a triplet of band indices $\{\boldsymbol{\nu} = (\nu_x, \nu_y, \nu_z)\}$. Whenever it is relevant, we use similar notations as for the fundamental band: For instance, Wannier functions in the band $\boldsymbol{\nu}$ are noted $w_{\boldsymbol{\nu}}$ and the annihilation operators $\hat{a}_{\boldsymbol{\nu},i}$. If only the fundamental band is relevant, we omit the band index to alleviate the notations. We gather all degenerate bands into "energy levels" indexed by an integer $\nu$. We neglect excited bands with $\nu_z \neq 0$ and group the first relevant bands according to $\nu = 0 \equiv \{\boldsymbol{\nu} = (0,0,0)\}$, $\nu = 1 \equiv \{\boldsymbol{\nu} = (1,0,0), (0,1,0)\}$, $\nu = 2 \equiv \{\boldsymbol{\nu} = (1,1,0), (2,0,0), (0,2,0)\}$, etc. Note that we assume a perfect symmetry between the two HL arms, which is verified in the experiment up to about 5 %.

### B. Bose-Hubbard model

The single-band Bose-Hubbard (BH) Hamiltonian describing our system is given in Eq. (1) of the main text. The harmonic potential takes the form $V_i = M(\Omega_x^2 x_i^2 + \Omega_y^2 y_i^2)/2$ with frequencies $\Omega_{x/y}$ arising from the Gaussian envelope of the lattice lasers [7, 8]. $M$ is the atomic mass.

The BH model is a good description of the experimental system for sufficiently high HL depths, roughly $V_\perp \gtrsim 5 - 6\,E_\mathrm{R}$ [8]. This criterion is mainly determined by two factors: the bandgap to higher excited bands must be much larger than the inverse of the intrinsic timescales in the lowest band (to justify the single-band description), and the tunneling energies beyond nearest neighbors must be much smaller than $J$ (to justify the tight-binding approximation). Taking $V_\perp \geq 6\,E_\mathrm{R}$ ensures that the two criteria are fulfilled by one order of magnitude or more. Data taken outside this range are stressed by a grey shaded area in the relevant figures of the Supplementary Information.

### C. Theoretical description of light scattering

#### 1. *Master equation for the ground state density matrix*

We consider a quantum gas of ultracold atoms with two internal states $g$ and $e$. The $g-e$ transition is driven by an off-resonant laser. In general, the dynamics of the laser driven atomic ensemble is described by a quantum master equation for the atomic density matrix [9–12]. We consider here the experimentally relevant limit of large detunings and weak saturation of the excited state. In this limit, the population in $e$ is negligible at all times, and the excited state can be eliminated adiabatically [9–11]. The evolution of the spatial coherences in the ground state is then governed by a master equation for the reduced ground state density matrix $\hat{\rho}$,

$$\frac{\mathrm{d}\hat{\rho}}{\mathrm{d}t} \approx \frac{1}{\mathrm{i}\hbar}\left[\hat{H}_0 + \hat{V}_\mathrm{dd}, \hat{\rho}\right] + \mathcal{L}[\hat{\rho}]. \tag{S1}$$

This describes the effect that off-resonant scattering of laser photons has on the quantized motional state of the gas.

The structure of Eq. (S1) is that of a Lindblad master equation describing Markovian open systems [13]. The commutator describing the unitary evolution involves the Hamiltonian $\hat{H}_0$ in the absence of laser light (including atom-atom interactions). In the presence of laser light, a dipole-dipole interaction term $V_\mathrm{dd}(\boldsymbol{r} - \boldsymbol{r}') \propto 1/|\boldsymbol{r} - \boldsymbol{r}'|^3$

also appears. Finally, the so-called Lindblad superoperator $\mathcal{L}$ describes relaxation of the atomic motional degrees of freedom due to spontaneous emission and collective effects. The dipole-dipole interaction $\hat{V}_{\rm dd}$ and the Lindblad dissipator are related to each other (see [12] and references therein). Explicit expressions for these operators are given in [12], and their origin discussed in detail.

#### 2. *Bose-Hubbard master equation*

The BH Hamiltonian in Eq. (1) of the main text is derived from a more general many-body Hamiltonian under the single-band and tight-binding assumptions [8]. Applying these assumptions to the ground state master equation (S1) [12], one finds a discretized version with the Hamiltonian $\hat{H}_0 \to \hat{H}_{\rm BH}$, and a Lindblad dissipator

$$\mathcal{L}[\hat{\rho}] = \frac{\gamma_{\rm sp}}{2}\sum_{i,j}\Lambda_{ij}\left(2\hat{n}_i\hat{\rho}\hat{n}_j - \hat{n}_i\hat{n}_j\hat{\rho} - \hat{\rho}\hat{n}_i\hat{n}_j\right), \quad \text{(S2)}$$

where $\hat{\rho}$ now denotes the projection on the fundamental band of the density matrix. The rates $\Lambda_{ij}$ are determined by the overlap integrals,

$$\Lambda_{ij} = \int {\rm d}^3\boldsymbol{r}{\rm d}^3\boldsymbol{r'}F(\boldsymbol{r}-\boldsymbol{r'})|w(\boldsymbol{r}-\boldsymbol{r}_i)|^2|w(\boldsymbol{r'}-\boldsymbol{r}_j)|^2. \quad \text{(S3)}$$

The kernel involves the Fourier tranform

$$F(\boldsymbol{r}-\boldsymbol{r'}) = \int {\rm d}^2\boldsymbol{u}\, D(\boldsymbol{u}){\rm e}^{{\rm i}\Delta\boldsymbol{k}\cdot(\boldsymbol{r}-\boldsymbol{r'})}, \quad \text{(S4)}$$

of the directional factor $D(\boldsymbol{u})$ describing the radiation pattern of the atomic dipole. This factor reads $D(\boldsymbol{u}) = (3/8\pi)\times[1-(\boldsymbol{u}\cdot\boldsymbol{\epsilon}_{\rm L})^2]$ for our choice of $\pi$-polarization (see Fig. 1). In Eq. (S4), the quantity $\Delta\boldsymbol{k} = \boldsymbol{k}_{\rm L} - k_0\boldsymbol{u}$ describes a “momentum kick” after absorbing a laser photon of momentum $\hbar\boldsymbol{k}_{\rm L}$ and spontaneously emitting a photon of momentum $\hbar k_0\boldsymbol{u}$, with $k_0 = 2\pi/\lambda_0$ and $\boldsymbol{u}$ a random unit vector corresponding to the direction of propagation.

Absorption-spontaneous emission cycles can be interpreted as weak, continuous measurements of the atoms' position at a rate $\gamma_{\rm sp}$ [14]. The motional degrees of freedom of the gas become entangled with the electromagnetic field when they interact, and erasing the information about the electro-magnetic field projects the atomic state into a state of ill-defined momentum, and therefore well-defined position by Heisenberg's principle. The function $F$ quantifies the resolution of this measurement: $F$ falls to zero for distances $\gg 1/k_0$, which is nothing but the diffraction limit associated with the optical detection of the atomic position.

#### 3. *Zero-range model*

The optical lattice spacing $d = \lambda_{\rm lat}/2$ and the range of $F$ are both on the order of an optical wavelength. In the BH regime, the Wannier functions are localized on a much smaller scale. When calculating the on-site decay rate $\Lambda_{ii}$, one can approximate $F(\boldsymbol{r}-\boldsymbol{r'}) \approx F(\boldsymbol{0}) = 1$ and $\Lambda_{ii} \approx F(\boldsymbol{0})$. Moreover, $F$ is maximal at the origin and the localization of Wannier functions near their respective centres implies that $|\Lambda_{i,j\neq i}| \ll |\Lambda_{ii}|$. This allows us to perform a so-called “zero-range approximation” in the following, where we retain only the on-site decay terms and neglect off-sites terms with $i \neq j$: $\Lambda_{ij} \approx \delta_{ij}$. Such an approximation becomes exact in the limiting case where the Wannier functions become infinitely localized, similar to the Lamb-Dicke limit where inter-band transitions are supressed. In the same limit, dipole-dipole interactions are no longer relevant: off-site terms are negligible and the on-site term can be absorbed in the on-site interaction energy $U$ of the BH Hamiltonian.

### D. Non-interacting atoms: quasi-momentum diffusion and inter-band transitions

#### 1. *Quasi-momentum diffusion in the fundamental band*

It is instructive to examine the solution of the master equation (S1) for $N$ non-interacting atoms. We consider for simplicity the tight-binding single-band BH model and use the zero-range approximation introduced before, thereby also neglecting dipole-dipole interactions and collective effects. The single-particle density matrix elements can be written $\rho_{i,j} = \langle w_i|\hat{\rho}|w_j\rangle$, where $|w_j\rangle$ denotes a state where the particle is located at site $j$ ($|w_j\rangle = |n_1 = 0, n_2 = 0, \cdots, n_j = 1, \cdots\rangle$ in Fock notation). The evolution equation for the density matrix elements is

$$\frac{{\rm d}\rho_{i,j}}{{\rm d}t} = \frac{1}{{\rm i}\hbar}\langle w_i|[\hat{H}_{\rm BH},\hat{\rho}]|w_j\rangle + \gamma_{\rm sp}\left(\delta_{ij}-1\right)\rho_{i,j}, \quad \text{(S5)}$$

where the coherent part involving the BH Hamiltonian reduces to the tunneling term. We quantify the evolution of spatial coherence using the spatially averaged first-order correlation function $C^{(1)}(j) = \sum_i \rho_{i,i+j}$. From Eq. (S5), we derive an equation of motion for $C^{(1)}$ for a uniform system with periodic boundary conditions,

$$\frac{{\rm d}C^{(1)}(j)}{{\rm d}t} = -\gamma_{\rm sp}C^{(1)}(j) + \gamma_{\rm sp}N\delta_{j0}. \quad \text{(S6)}$$

For $j = 0$, this equation simply expresses the conservation of atom number. For $j \neq 0$, it shows that the spatial coherences decay exponentially at a rate $\gamma_{\rm sp}$.

We calculate the quasi-momentum distribution $\mathcal{P}(p) = (1/N_{\rm s})\sum_j C^{(1)}(j){\rm e}^{{\rm i}pj}$ as the Fourier transform of $C^{(1)}$, with $p$ in units of the fundamental lattice wavevector $2k_{\rm lat}$ and $N_{\rm s}$ the number of sites. We then get

$$\frac{{\rm d}\mathcal{P}(p)}{{\rm d}t} = -\gamma_{\rm sp}(\mathcal{P}(p) - \bar{n}), \quad \text{(S7)}$$

where $\bar{n} = N/N_{\rm s}$ is the filling factor. The explicit solution is Eq. (1) in the main text [15],

$$\mathcal{P}(p,t) = \mathcal{P}(p,t=0)\mathrm{e}^{-\gamma_{\rm sp}t} + \bar{n}(1-\mathrm{e}^{-\gamma_{\rm sp}t}). \tag{S8}$$

The width of the quasi-momentum distribution evolves according to

$$\Delta p^2 = \Delta p_0^2 \mathrm{e}^{-\gamma_{\rm sp}t} + \Delta p_\infty^2(1-\mathrm{e}^{-\gamma_{\rm sp}t}). \tag{S9}$$

Here $\Delta p_\infty^2$ corresponds to the final width of the uniform distribution $\mathcal{P}(p,\infty) = \bar{n}$. For the case where the initial state is the $p=0$ Bloch state, $\Delta p_0 = 0$, the momentum distribution exhibits a diffusive behavior with $\Delta p \propto \sqrt{t}$ for short times $\gamma_{\rm sp}t \ll 1$.

#### 2. *Inter-band transitions*

Our discussion has so far been restricted to single-band dynamics, even though photon scattering inherently redistributes momentum and triggers inter-band transitions. In the experiment, the excitation laser propagates vertically but the VL is set much deeper than the HL to limit inter-band transitions in that direction. The importance of these transitions can be quantified by evaluating the Lamb-Dicke parameters

$$\eta_{\perp/z} = \frac{\int \mathrm{d}^2\boldsymbol{u} D(\boldsymbol{u}) \left|\langle w_{\perp/z}|\mathrm{e}^{\mathrm{i}\Delta\boldsymbol{k}\cdot\hat{\boldsymbol{r}}}|w_0\rangle\right|^2}{\int \mathrm{d}^2\boldsymbol{u} D(\boldsymbol{u}) \left|\langle w_0|\mathrm{e}^{\mathrm{i}\Delta\boldsymbol{k}\cdot\hat{\boldsymbol{r}}}|w_0\rangle\right|^2}, \tag{S10}$$

where $D(\boldsymbol{u}) = (3/8\pi) \times [1-(\boldsymbol{u}\cdot\boldsymbol{\epsilon}_{\rm L})^2]$ is the radiation pattern of the atomic dipole. The factors $\eta_{\perp/z}$ correspond to the probability per spontaneous emission to undergo band-changing transitions from the fundamental band $\nu = 0$ with Wannier function $|w_0\rangle$ to one of the first degenerate excited bands $\nu = 1$ (subscript $\perp$) or $\boldsymbol{\nu} = (0,0,1)$ (subscript $z$) with Wannier function $|w_{\perp/z}\rangle$. For the experimental parameters used in the main text we find $\eta_z \approx 0.2$ and $\eta_\perp \approx 0.1$. As a result of the vertical integration by the probe beam we do not resolve the band dynamics in the vertical direction.

### E. Two atoms and two wells

We illustrate the influence of interactions on the dissipative model in the simplest case with two atoms and two lattice sites. The bosonic Hilbert space is spanned by only three states, that can be taken to be $\{|S\rangle, |I\rangle, |A\rangle\}$, with the two symmetric and antisymmetric combinations $|S/A\rangle = (|2,0\rangle \pm |0,2\rangle)/\sqrt{2}$ and $|I\rangle = |1,1\rangle$, with $|n,m\rangle$ a Fock state with $n$ atoms in the left (L) well and $m$ in the right (R) one. In this basis, the Bose-Hubbard Hamiltonian reads

$$\hat{H} = U\left(|S\rangle\langle S| + |A\rangle\langle A|\right) - 2J\left(|I\rangle\langle S| + |S\rangle\langle I|\right). \tag{S11}$$

We now consider the dissipative evolution described by Eq. (S1). The dynamics can be analyzed conveniently using the formalism of quantum Monte-Carlo trajectories [13, 16]. To this end we rewrite the master equation as

$$\frac{\mathrm{d}}{\mathrm{d}t}\hat{\rho} = \frac{1}{\mathrm{i}\hbar}\left[\hat{H},\hat{\rho}\right] + \frac{\gamma_{\rm sp}}{2}\left(\hat{\Delta}\hat{\rho}\hat{\Delta} - \frac{1}{2}\hat{\Delta}^2\hat{\rho} - \frac{1}{2}\hat{\rho}\hat{\Delta}^2\right) \tag{S12}$$

$$= \frac{1}{\mathrm{i}\hbar}\left(\hat{H}_{\rm eff}\hat{\rho} - \hat{\rho}\hat{H}_{\rm eff}^\dagger\right) + \hat{\mathcal{J}}\left[\hat{\rho}\right], \tag{S13}$$

with the number difference operator $\hat{\Delta} = \hat{n}_{\rm L} - \hat{n}_{\rm R}$. We introduced an effective Hamiltonian

$$\hat{H}_{\rm eff} = \hat{H} - \frac{\mathrm{i}\hbar\gamma_{\rm sp}}{4}\hat{\Delta}^2, \tag{S14}$$

and a jump operator

$$\hat{\mathcal{J}}\left[\hat{\rho}\right] = \frac{\gamma_{\rm sp}}{2}\hat{\Delta}\hat{\rho}\hat{\Delta}. \tag{S15}$$

In the Monte-Carlo picture, the dissipative evolution in an infinitesimal time interval $[t, t+\delta t]$ is stochastic. The system either stays in the state $|\Psi(t)\rangle$ evolved under the effective Hamiltonian, or undergoes a quantum jump to the (unnormalized) state $\hat{\Delta}|\Psi(t)\rangle$ with probability $\delta p = \gamma_{\rm sp}\delta t\langle\Psi(t)|\hat{\Delta}^2|\Psi(t)\rangle/2$.

In the limit $J \to 0$, quantum jumps change the symmetric to the antisymmetric state and reciprocally (thereby randomizing the relative phase), but do not occur for the Fock state $|I\rangle$. When $J \neq 0$, the antisymmetric state $|A\rangle$ remains an eigenstate of $\hat{H}_{\rm eff}$ with eigenvalue $U - \mathrm{i}\hbar\gamma_{\rm sp}$. The other two eigenstates are superpositions $|\pm\rangle = a_\pm|I\rangle + b_\pm|S\rangle$ of $|I\rangle$ and $|S\rangle$ with eigenvalues

$$E_\pm = \frac{U - \mathrm{i}\hbar\gamma_{\rm sp}}{2} \pm \frac{1}{2}\sqrt{U^2 - (\hbar\gamma_{\rm sp})^2 + 16J^2 - 2\mathrm{i}U\hbar\gamma_{\rm sp}}. \tag{S16}$$

In the limit $U \to +\infty$, the eigenvalues become

$$E_+ \approx U - \mathrm{i}\hbar\gamma_{\rm sp} + \frac{4J^2}{U}, \qquad E_- \approx -\frac{4J^2}{U} - \mathrm{i}\frac{4J^2\hbar\gamma_{\rm sp}}{U^2}, \tag{S17}$$

where we restricted the expansions of the real and imaginary parts to leading orders in $J, \gamma_{\rm sp}$. We thus find that the lowest energy state $|-\rangle$ ($|G\rangle$ in the main text) relaxes with a rate $\sim \gamma_{\rm sp}(2J/U)^2$, much slower than $\gamma_{\rm sp}$ due to the strong on-site interaction. In contrast, the two other states $|A\rangle$ and $|+\rangle$ relax with a rate $\sim \gamma_{\rm sp}$.

## III. ANALYSIS OF A CONTINUOUS MEASUREMENT MODEL

### A. Single-band zero-range model

We now turn to the analysis of the many-body model defined by the BH master equation. The Hamiltonian part $\hat{H}_0$ is the BH model (Eq. (1) in the main text) and the dissipation superoperator is, combining the single-band and zero-range approximations,

$$\mathcal{L}\left[\hat{\rho}\right] = \frac{\gamma_{\rm sp}}{2}\sum_i 2\hat{n}_i\hat{\rho}\hat{n}_i - \hat{n}_i^2\hat{\rho} - \hat{\rho}\hat{n}_i^2. \tag{S18}$$

This model was studied in detail by Poletti *et al.* in [17, 18]. We recall that collective effects (super- or sub-radiance, light-induced dipole-dipole interactions) and inter-band transitions are neglected [12]. As a result, the model of [17, 18] should be viewed as the minimal description of a dissipative BH system submitted to continuous measurement by light scattering. Yet, as we argue in the main article and below, the model captures the essential features of the non-trivial momentum diffusion observed in our experiments.

The density matrix can be represented in the Fock basis as $\hat{\rho} = \sum_{\boldsymbol{n},\boldsymbol{m}} \rho_{\boldsymbol{m}}^{\boldsymbol{n}} |\boldsymbol{n}\rangle\langle\boldsymbol{m}|$, where $\boldsymbol{n} = (n_1, \cdots, n_{N_s})$ identifies a particular configuration of Fock states on the $N_s$ sites. Statistical mixtures of Fock states are not affected by dissipation due to the particular structure of $\mathcal{L}$, and for finite tunneling there exists a unique asymptotic steady-state $\rho_{\boldsymbol{m}}^{\boldsymbol{n}} \propto \delta_{\boldsymbol{m},\boldsymbol{n}}$, a fully mixed state where all Fock state configurations are equally likely [18].

A key observation of Poletti *et al.* [17, 18] is that the relaxation to the steady-state proceeds *via* three stages:

- an initial stage governed by the time scale $\gamma_{sp}^{-1}$, where the number distribution broadens and the long-range coherence potentially present in the initial state decays exponentially [10],
- an intermediate stage, where relaxation slows down dramatically and an algebraic regime emerges. This regime corresponds to a state which essentially belongs to a decoherence-free subspace and does not decay. Finite tunneling amplitude partially restores coherence in this mixture of Fock states ("quantum fluctuations around the decoherence free subspace") and allows relaxation to persist in a strongly modified manner,
- a final stage where the system "thermalizes" towards the asymptotic steady-state.

The first regime where long-range coherence disappears can not be precisely described by the formalism of [17, 18], and we did not attempt to do it theoretically. However, we provide an empirical discussion of the experimentally observed behavior in Sec. VI C.

### B. Anomalous diffusion in the algebraic regime

#### 1. *Master equation for populations*

In the second stage of the decay, coherence is already short-ranged. The density matrix is mainly diagonal with a weak contribution of the off-diagonal coherences $\rho_{\boldsymbol{n}}^{\boldsymbol{n}+\boldsymbol{e}_{i,j}}$ between configurations differing by one tunneling event with $i, j$ nearest-neighbors. The vector $\boldsymbol{e}_{i,j}$ with components $(\boldsymbol{e}_{i,j})_k = +1$ if $k = i$, $-1$ if $k = j$, and 0 otherwise indicates that we consider a process where one atom moved from site $j$ to site $i$. We neglect other off-diagonal matrix elements between configurations differing by two or more tunneling events.

Because of the large mismatch between interaction energy and damping rate, the rapidly-oscillating coherence can be expressed as a slave variable depending on the slowly-evolving populations. Following Poletti *et al.* [18], the steady-state coherences are given by

$$\rho_{\boldsymbol{n}}^{\boldsymbol{n}+\boldsymbol{e}_{i,j}} \approx \frac{J\sqrt{n_j(n_i+1)}}{U(n_i-n_j+1)+\mathrm{i}\hbar\gamma_{sp}} \left(\rho_{\boldsymbol{n}}^{\boldsymbol{n}} - \rho_{\boldsymbol{n}+\boldsymbol{e}_{i,j}}^{\boldsymbol{n}+\boldsymbol{e}_{i,j}}\right). \quad \text{(S19)}$$

Adiabatic elimination of the coherences leads to a set of closed equations of motion for the populations $\rho_{\boldsymbol{n}}^{\boldsymbol{n}}$ alone, valid in the limit $U, \hbar\gamma_{sp} \gg J$ where the populations relax much more slowly than the coherences (Equation 3S in the Supplementary Material of [18]).

An additional simplification comes from assuming a factorization ansatz for the dominant diagonal part of the density matrix,

$$\hat{\rho} \approx \prod_i \left( \sum_{n_i=0}^{\infty} p_{n_i} |n_i\rangle_i\,{}_i\langle n_i| \right). \quad \text{(S20)}$$

With this additional assumption, the complicated evolution equation for the diagonal matrix elements reduces to a difference equation obeyed by the on-site number distribution $p_n$ [18],

$$\frac{\mathrm{d}p_n}{\mathrm{d}\tau} = W_{n+1}(p_{n+1}-p_n) - W_{n-1}(p_n - p_{n-1}). \quad \text{(S21)}$$

Here we introduced the rescaled time $\tau = t/t^*$, with the characteristic interaction-enhanced time

$$t^* = \frac{1}{2z\gamma_{sp}} \left(\frac{U\bar{n}}{J}\right)^2 \gg \gamma_{sp}^{-1}, \quad \text{(S22)}$$

and with $\bar{n}$ the average filling and $z$ the number of nearest neighbors. The master equation (S21) is governed by the non-linear transition rates

$$W_{n+1} = \bar{n}^2 \sum_m g(n+1, m) p_{m-1}, \quad \text{(S23)}$$

$$W_{n-1} = \bar{n}^2 \sum_m g(n, m+1) p_{m+1}, \quad \text{(S24)}$$

where the function $g$ is defined as

$$g(x, y) = \frac{xy}{(x-y)^2 + (\hbar\gamma_{sp}/U)^2}. \quad \text{(S25)}$$

The characteristic time $t^*$ allows us to identify the three regimes described earlier: *(i)* $t \lesssim \gamma_{sp}^{-1}$: initial relaxation of coherences, *(ii)* $\gamma_{sp}^{-1} \lesssim t \ll t^*$: algebraic regime, *(iii)* $t \gtrsim t^*$: final relaxation to the steady-state.

#### 2. *Scaling regime*

Poletti *et al.* [18] solved the master equation numerically using an array of Fock states as initial condition. They pointed out that the number distribution obeys

scale invariance for specific conditions, namely in a "scaling window" $\gamma_{\rm sp}^{-1} \lesssim t \ll t^*$ such that $\Delta n(t) \ll \bar{n}$.

This scale invariance characterizes the algebraic regime and can be justified in the limit of large fillings $\bar{n} \gg 1$ and weak dissipation $\hbar\gamma_{\rm sp}/U \to 0$. This allows one to make a continuum approximation where the discrete variable $n$ is replaced by a continuous one $x = n/\bar{n} \in [0, \infty[$. The discrete occupation number distribution becomes continuous, $p_n \longrightarrow p(x)/\bar{n}$, and the master equation maps to a Fokker-Planck equation with a non-linear diffusion term [17, 18]. With an initial Fock state $p_n = \delta_{n,\bar{n}}$ [$p(x) \propto \delta(x-1)$] and for weak dissipation, there exists a solution which exhibits scale invariance,

$$p(x) \approx \frac{1}{\tau^\beta} f\left(u = \frac{x-1}{\tau^\beta}\right), \qquad \text{(S26)}$$

with a normalized time $\tau$ and a scaling exponent $\beta$ [18]. The scaling function is

$$f(u) = \frac{1}{4\Gamma(5/4)} \mathrm{e}^{-u^4/16}, \qquad \text{(S27)}$$

where $\Gamma$ denotes the Gamma function and where the scaling exponent is $\beta = 1/4$ [18].

This scaling solution is only exact in the limit defined by $\hbar\gamma_{\rm sp}/U \ll 1$ and $\bar{n} \gg 1$. However, it remains relevant outside the high-filling limit provided two conditions are met. First, the average filling $\bar{n}$ must not be too small, and second, the number distribution must be peaked around $\bar{n}$ with small dispersion $\Delta n \ll \bar{n}$. With these conditions fulfilled, the numerical solutions of the master equation (S21) approximately obey the scaling form until the second condition gets violated for times $t \approx t^*$ [18]. This defines a "scaling window" in the time evolution, roughly determined by $\gamma_{\rm sp}^{-1} \lesssim t \ll t^*$. The width of this windows shrinks with decreasing filling or increasing initial number fluctuations, until $\gamma_{\rm sp} t^* \sim 1$ and the scaling behavior essentially disappears. For a system described by the BH model, number squeezing occurs even in the superfluid regime where $\Delta n \sim 1$ as soon as $U \gtrsim J$. As a result, the scaling behavior starts being observable for fillings as low as $\bar{n} \gtrsim 1.5$. We discuss in the following section that this behavior, first noticed in [18] for the evolution of $p_n$, is also visible in the evolution of the spatial coherence.

## C. Nearest-neighbor coherence

### 1. *General formula in the algebraic regime*

We now evaluate how phase coherence evolves in the algebraic regime. Initially, the gas could possess long-range correlations that decay in the first stage of the evolution. In the algebraic stage, correlations are short-ranged and dominated by the nearest-neighbor correlation function $C_{\pm1} = \langle \hat{a}_{i\pm1}^\dagger \hat{a}_i \rangle$. One can relate this correlation function to the density matrix elements,

$$C_{\pm1} = \sum_{\boldsymbol{n}} \sqrt{n_i(n_{i\pm1}+1)}\, \rho_{\boldsymbol{n}}^{\boldsymbol{n}+\boldsymbol{e}_{i\pm1,i}}. \qquad \text{(S28)}$$

Using the nearest-neighbor coherences in Eq. (S19) and the factorization ansatz in Eq. (S20), we find

$$C_{\pm1} = \frac{J}{U} \sum_{m,n=0}^{+\infty} (n-m) g(m+1, n+1) [p_n p_{m+1} - p_{n+1} p_m], \qquad \text{(S29)}$$

the form we use for numerical calculations.

In Fig. S2 we show the solution of Eq. (S29) for various initial occupation probability distributions. A true scaling regime, reaching the universal limit of Eq. (S32), appears already for $\bar{n} > 1$ but only when $\Delta n \ll \bar{n}$.

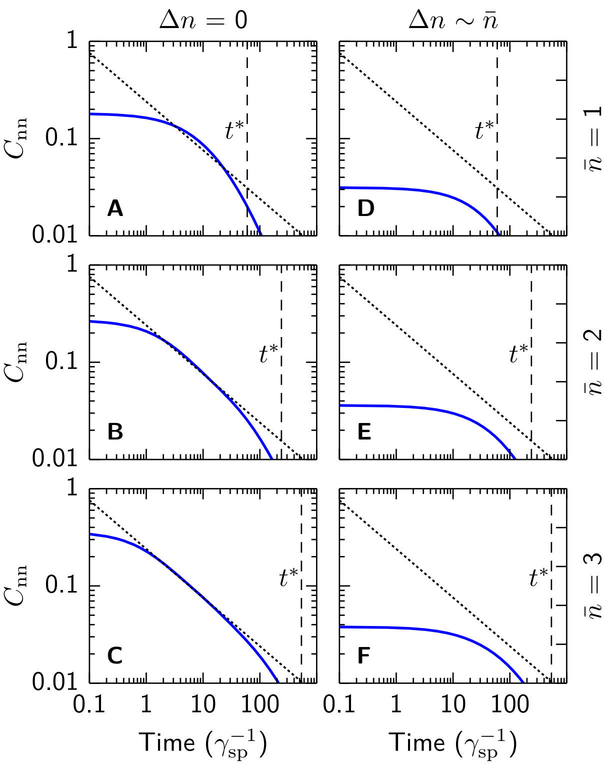


FIG. S2. **Emergence of a scaling regime in the dissipative BH model.** (**A** to **F**) Calculated time evolution of the nearest-neighbor coherence $C_{\rm nn}$ from Eq. (S29) (solid line), for $\bar{n} = 1$, 2 and 3. The dotted line is the universal form of Eq. (S32) valid for large fillings. The vertical dashed line shows the time $t^*$ from Eq. (S22). The BH parameters are calculated for $V_\perp = 10\,E_{\rm R}$. The initial distribution corresponds to a Fock state in (A) to (C) and to a coherent state in (D) to (F).

### 2. *Universal power-law decay for weak dissipation*

We can derive an analytical prediction in the limit of high fillings ($\bar{n} \gg 1$) and weak dissipation ($\gamma_{\rm sp}/U \to$

0). By taking the continuum limit in Eq. (S29), we find that the nearest-neighbor coherence factors $C_{\pm 1}$ take the following form in the scaling regime:

$$C_{\pm 1} \approx \frac{J\eta_0}{U\tau^{\alpha}}. \tag{S30}$$

The nearest-neighbor coherence therefore inherits the scaling properties of the number distribution function $p$ but with a scaling exponent $\alpha = 2\beta = 1/2$ twice as large. The numerical factor $\eta_0 \approx 0.676$ is

$$\eta_0 = \int \mathrm{d}u\mathrm{d}v \frac{f(u)f'(v) - f'(u)f(v)}{u-v} = \frac{2\Gamma(3/4)}{\Gamma(1/4)}, \tag{S31}$$

where $\Gamma$ denotes the Gamma function. The coherence factor can be rewritten in the universal form quoted in the main text,

$$C_{\mathrm{nn}} = \frac{C_{\pm 1}}{\bar{n}} \approx \frac{0.478}{\sqrt{z\gamma_{\mathrm{sp}}t}}, \tag{S32}$$

which is independent of the microscopic parameters $U$, $J$ or $\bar{n}$.

## IV. LIGHT-INDUCED INELASTIC LOSSES

We observe atom losses in parallel with the loss of coherence when the dissipation laser is enabled, as illustrated in the main article. We attribute these losses to two-body light-assisted inelastic collisions of cold atoms in presence of a light field, as observed in numerous circumstances, including magneto-optical traps [19], off-resonant optical traps [20, 21], BEC superradiance [22] or quantum gas microscopes [23, 24]. In this section, we first describe and complete the analysis presented in the main article, and finally comment on the order of magnitude of the measured loss rate.

### A. Scaling behavior in the loss dynamics

We fit the atom number decay using an *ad hoc* function that reproduces well the observed behavior,

$$N = \frac{N_0}{1 + (\gamma_{2\mathrm{B}} t)^{\beta}}. \tag{S33}$$

We show the best-fit parameters in Fig. S3 (black circles). The fitted exponent $\beta$ approaches a constant value $\sim 1/2$ (Fig. S3A) for lattice depths $V_\perp \gtrsim 5\,E_{\mathrm{R}}$.

In Fig. S3B, we show that the ratio $\hbar\gamma_{2\mathrm{B}}/U$ between the fitted two-body loss rate and the on-site interaction energy $U$ saturates to a constant value $\approx 0.1$ for lattice depths above $5\,E_{\mathrm{R}}$. In the BH regime, the atom number decay is governed by a strictly local rate equation of the form

$$\frac{\mathrm{d}\bar{n}_i}{\mathrm{d}t} = -\gamma_{2\mathrm{B}} \langle \hat{n}_i(\hat{n}_i - 1)\rangle, \tag{S34}$$

with $\bar{n}_i = \langle \hat{n}_i \rangle$ the mean density and

$$\gamma_{2\mathrm{B}} = K_2 \int \mathrm{d}^3\boldsymbol{r}\, |w(\boldsymbol{r})|^2 = \frac{MK_2}{4\pi\hbar^2 a} U. \tag{S35}$$

Here $K_2$ is a two-body inelastic rate constant, and we emphasized that the ratio $\hbar\gamma_{2\mathrm{B}}/U$ is independent of the HL depth $V_\perp$. This matches our observations for $V_\perp \geq 5\,E_{\mathrm{R}}$, where the BH description is justified. For lower lattice depths, the assumption of strictly local losses underlying the BH description starts to break down: Additional terms not included in Eq. (S34) (for instance, involving nearest-neighbor density correlations $\propto \langle \hat{n}_i \hat{n}_j \rangle$, or density-induced tunneling $\propto \langle \hat{a}_i^\dagger \hat{n}_i \hat{a}_j \rangle$) start playing a role in the decay. These additional processes are effectively taken into account in the fitted loss rates. This explains the apparent increase of $\gamma_{2\mathrm{B}}$ for $V_\perp \leq 5\,E_{\mathrm{R}}$, which should rather be taken as an artifact of the BH description for low lattice depths.

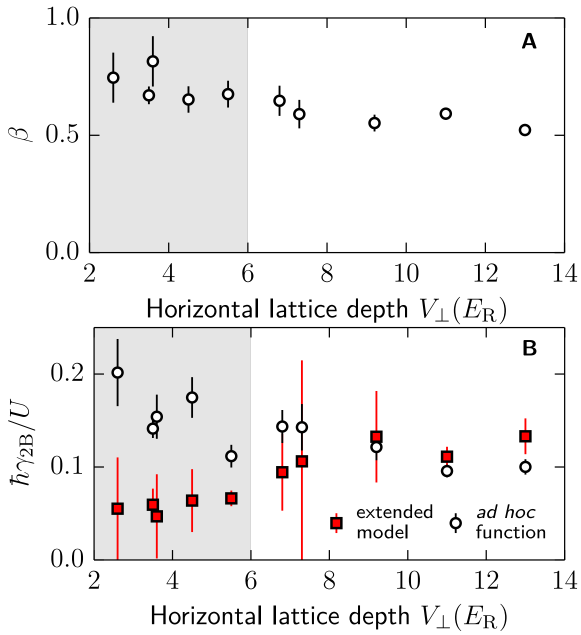


FIG. S3. **Analysis of atom losses.** (**A**) Fitted exponent for the atom number time evolution using Eq. (S33) versus HL depth. The exponent converges to $\beta = 1/2$ for HL depths $V_\perp \gtrsim 6\,E_{\mathrm{R}}$. (**B**) Two-body loss rate determined using the *ad hoc* function in Eq. (S33) (empty circles) or our extended model presented in Sec. V (filled squares) versus HL depth. The shaded areas shows the region where the BH model is not a valid description. Error bars are 1-sigma confidence intervals derived from a $\chi^2$ fitting procedure.

We present in Sec. V an extended model including inhomogeneities and losses. Using $\gamma_{2\mathrm{B}}$ as a free parameter in this extended model provides an independent determination (squares in Fig. S3B). Both sets of fitted values based either on the empirical Eq. (S33) or on the extended model are consistent with each other in the BH regime.

### B. Interpretation of the loss dynamics

Let us focus on the regime where the BH description holds, and also assume that the two-body correlation function entering Eq. (S34) is of the form $\langle \hat{n}_i(\hat{n}_i-1)\rangle = \bar{n}_i^2 h(t)$, where $h$ depends on time but not on the density $\bar{n}$. Integration of Eq. (S34) is straightforward for a uniform system, giving the decay law

$$\bar{n}_i(t) = \frac{\bar{n}_{i,0}}{1+\gamma_{2\mathrm{B}}\bar{n}_{i,0}H(t)}, \tag{S36}$$

with $H(t)=\int_0^t h(t')\mathrm{d}t'$ a primitive of $h$.

We now consider a two-dimensional system in a harmonic trap, as in our experiment, where the local density approximation applies. The initial density then obeys a law of the form $\bar{n}_{i,0} = n_0(x_i)$ with a reduced variable $x_i = (\mu - M\Omega_\perp^2 d^2 \boldsymbol{r}_i^2/2)/U$. Here $\mu$ is the chemical potential, $\Omega_\perp$ the trap frequency and $\boldsymbol{r}_i$ the position of site $i$ in units of $d$. Taking a continuum limit, the atom number $N(t)=\sum_i \bar{n}_i$ obeys

$$N(t) = \frac{2\pi U}{M\Omega_\perp^2 d^2}\int_0^{x_0}\mathrm{d}x\,\frac{n_0(x)}{1+\gamma_{2\mathrm{B}}n_0(x)H(t)}, \tag{S37}$$

with $x_0=\mu/U$. When $t\to\infty$, we find that the atom number decays according to the asymptotic law

$$N(t)\to 2\pi\frac{U}{\gamma_{2\mathrm{B}}}\frac{x_0}{M\Omega_\perp^2 d^2}\frac{1}{H(t)}. \tag{S38}$$

The asymptotic decay depends weakly on the lattice depth: $U/\gamma_{2\mathrm{B}}$ depends only on atomic properties (see previous paragraph), and $x_0/M\Omega_\perp^2 d^2 \approx 2000/E_\mathrm{R}$ typically varies very little with the lattice depth.

We discuss in the main article that we observe a decay law empirically captured by Eq. (S33). From the previous discussion, we infer that this decay law would correspond to a two-body correlation function $\langle \hat{n}_i(\hat{n}_i-1)\rangle \propto 1/\sqrt{t}$. Asymptotically, the two-body correlation function $\langle \hat{n}_i(\hat{n}_i-1)\rangle$ vanishes. A system of hardcore bosons where only empty or singly-occupied sites are allowed is an asymptotic state compatible with this behavior: Since $\bar{n}_i = p_1 = 1-p_0$ and $\langle \hat{n}_i^2\rangle = p_1$ for hardcore bosons, one necessarily has $\langle \hat{n}_i(\hat{n}_i-1)\rangle = 0$. A possible interpretation is thus that the system is driven to such a hardcore bosons state by inelastic losses. This scenario is reminiscent of an experiment performed on molecules in a one-dimensional optical lattice [25].

### C. Estimation of the semi-classical loss rate

We now discuss the order of magnitude of the two-body light-induced loss rate. Microscopically, these losses originate from collisions between one atom in the ground state $g$ and one in the excited state $e$. The interaction potential between the atoms is dominated at large distance by a $C_3/r_{eg}^3$ dipole-dipole interaction, where the $C_3$ coefficient can be either negative (attractive branches) or positive (repulsive branches).

Attractive branches usually support several molecular bound states. Photoassociation resonances to such states have been reported for $^{174}$Yb in [26, 27]. They are located at negative detunings from the inter-combination transition, with the resonance closest to the dissociation threshold at $-4.2\,$MHz from the transition. For our laser detuning $\delta_\mathrm{L} = +15\Gamma_0$, the two-body loss rate $K_2^\mathrm{PA}$ induced by this photoassociation resonance [27] is $K_2^\mathrm{PA} n_0/\gamma_\mathrm{sp} \approx 10^{-3}$ for the densities $n_0 \approx 10^{14}\,\mathrm{cm}^{-3}$ explored in our experiment. We thus conclude that off-resonant photoassociation plays a negligible role.

The blue-detuned laser can however resonantly excite the repulsive branches in the interaction potential [28, 29]. We used the semi-classical calculation of [30] to provide an estimate on the inelastic collision rate $K_2$ caused by the repulsive branches. We find $K_2 \leq 2\gamma_\mathrm{sp}\lambda_0^3/(9\pi) \approx 5\times 10^{-12}\,\mathrm{at/cm^3/s}$. We thus find

$$\frac{\hbar\gamma_{2\mathrm{B}}}{U} = \frac{MK_2}{4\pi\hbar a} \leq 0.19. \tag{S39}$$

This agrees well with the order of magnitude measured experimentally (see Fig. S3B).

## V. EXTENDED MODEL: EXTERNAL CONFINEMENT AND LOSSES

In the experiment, the density distribution is inhomogeneous due to the auxiliary trapping potential provided by the lattice beams envelopes. Moreover the total atom number decreases with time, because of light-assisted inelastic losses. For a faithful simulation of the actual dissipative dynamics, we take these two aspects into account.

### A. Inhomogeneous density distribution

The model studied in [18] focuses on uniform systems prepared in a Mott insulator state with integer filling $\bar{n}$, whereas our experimental situation is more complex because of an additional harmonic potential created by the lattice beams. This leads to an inhomogeneous spatial distribution of $\bar{n}$ with a maximum value around 2.5 in the center of the cloud. Morever, we probe a many-body ground state which is not a Mott insulator state. We thus extend the model by taking into account the inhomogeneity and the initial ground state.

We use a similar approach as in [2] to predict the initial equilibrium density distribution of atoms in the optical lattice. To compute the number of atoms in each plane of the VL, we model the first phase of our loading sequence using a sudden approximation. The atomic distribution for a BEC in the crossed optical dipole trap is projected on a periodic potential of period $d$ much smaller than the Thomas-Fermi half-length $L$ of the BEC. For a BEC

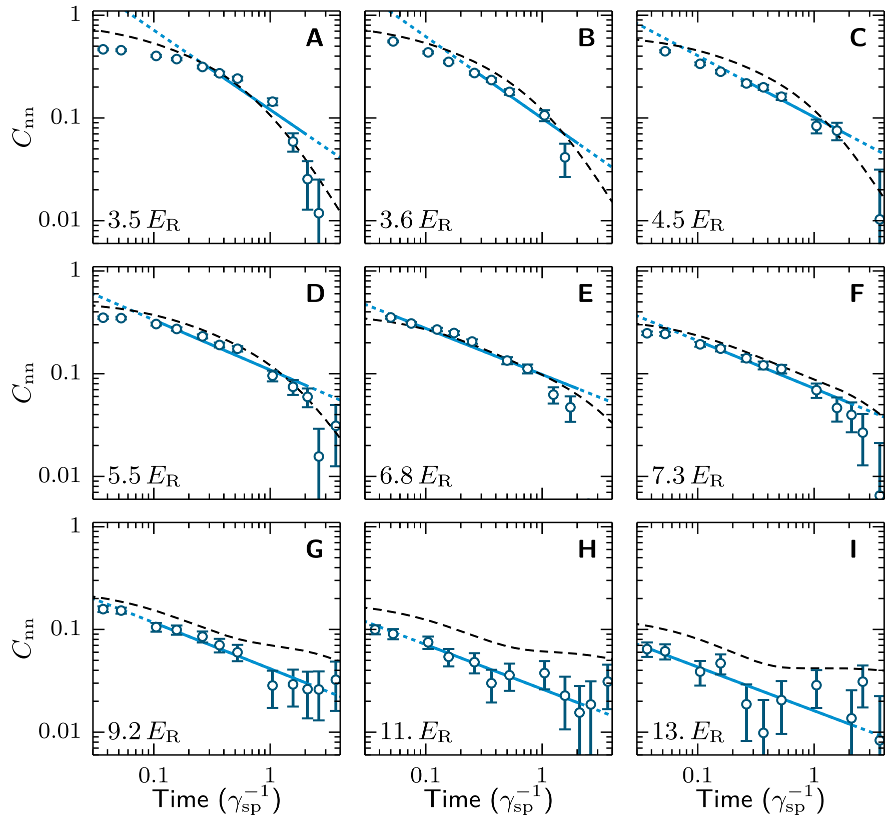


FIG. S4. **Nearest-neighbor coherence $C_{nn}$: full data set.** (**A** to **I**) Time evolution of $C_{nn}$, for all lattice depths $V_\perp$. $C_{nn}$ is obtained from fits as described in Sec. VI B. Solid lines show a fit to a power-law decay with exponent $\alpha$. Dashed lines show the prediction from our model presented in Sec. V. Error bars are 1-sigma confidence intervals derived from a $\chi^2$ fitting procedure.

in the Thomas-Fermi regime [31], this results in a distribution of atoms per plane $N_{i_z} \approx (15Nd/16L)\Upsilon(1-\tilde{z}^2)$. Here we used the notations $\Upsilon = x^2\Theta(x)$, with $\Theta$ the Heaviside step function, $\tilde{z} = 2i_z/N_{\rm pl}$ for the reduced vertical coordinate, and $N_{\rm pl} = 2L/d$ for the number of occupied planes in our model. The chemical potential in each plane is determined self-consistently so that the atom number is $N_{i_z}$. We then assume that the quantum gases in each plane can be described by the ground state of the BH model. The external trapping frequencies are given by $\Omega_i^2 = a_i^2 V_\perp/E_{\rm R} + b_i^2 V_z/E_{\rm R}$, with $a_{x,y,z} = 2\pi \times \{5.9, 5.4, 8.0\}$ Hz, $b_{x,y,z} = 2\pi\times\{4.5, 4.5, 0.0\}$ Hz and $V_z \approx 27\,E_{\rm R}$. We use the local density approximation to calculate the local chemical potential in each site and to compute the initial occupation probability distribution $p(n_i)$ using a Gutzwiller wavefunction [5–7].

For each site, we solve the model from Eq. (S21) using its initial occupation probability distribution. We then compute $C_{nn}$ by averaging Eq. (S29) over the spatial density profile. The final results are qualitatively the same as in the homogeneous case studied previously: The scaling regime and the associated universal law $C_{nn} \propto 1/\sqrt{t}$ appear for a narrow enough occupation number distribution $\Delta n \ll \bar{n}$ and for a sufficiently high filling $\bar{n} \gtrsim 1.5$. To explain the survival of the scaling behavior of $C_{nn}$ upon spatial averaging, we notice that *(i)* the less dense parts of the cloud where the scaling regime is never reached decay exponentially and their contribution to the correlation function quickly becomes negligible, and that *(ii)* the denser parts do obey scaling and follow Eq. (S32) which is independent of the density.

### B. Including atom losses

While the model of [18] captures the power-law behavior and the exponent observed experimentally, it also predicts a much slower decay than in the experiments. The timescale $t^* \propto (U/J)^2$ governing the duration of the scaling window with algebraic decay changes by several orders of magnitude when $V_\perp$ varies from 3 to 13 $E_{\rm R}$. In the experiments, we observe instead that the correlation function decays on a timescale $\sim \gamma_{\rm sp}^{-1}$ for all lattice depths (up to a numerical factor). We resolve this discrepancy by considering the effect of inelastic losses on the decay of coherence.

To include the observed two-body losses in the theory, we add another Lindblad superoperator

$$\mathcal{L}_{2B}[\hat{\rho}] = \frac{\gamma_{2B}}{2}\sum_i 2\hat{a}_i^2\hat{\rho}\hat{a}_i^{\dagger 2} - \hat{a}_i^{\dagger 2}\hat{a}_i^2\hat{\rho} - \hat{\rho}\hat{a}_i^{\dagger 2}\hat{a}_i^2 \qquad \text{(S40)}$$

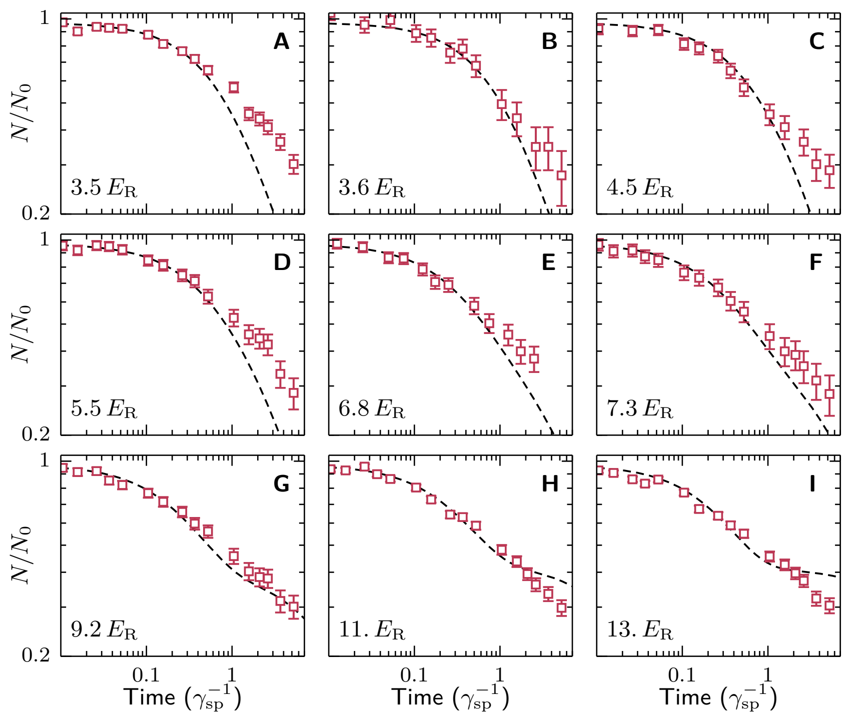


FIG. S5. **Atom number $N$: full data set.** (**A** to **I**) Time evolution of $N$ for all lattice depths $V_\perp$. Dashed lines show the prediction from our model presented in Sec. V. Error bars are 1-sigma confidence intervals derived from a $\chi^2$ fitting procedure.

to the master equation (S1), with a two-body loss rate $\gamma_{2B} \propto U$. $\mathcal{L}_{2B}$ couples configurations with different atom numbers (unlike $\mathcal{L}$), making a direct extension of the theory not trivial. If $\gamma_{2B}$ is smaller than the spontaneous emission rate, the coherences evolve essentially as in the lossless case, with a small correction due to inelastic decay. If we neglect this correction and apply the same procedure as without losses, we obtain a master equation for populations with an additional two-body loss term in the master equation (S21),

$$\left.\frac{\mathrm{d}p_n}{\mathrm{d}t}\right|_{\mathrm{losses}} = -\gamma_{2B} n(n-1)p_n + \gamma_{2B}(n+2)(n+1)p_{n+2}. \tag{S41}$$

We extended the model of Sec. III using Eq. (S41), even though the condition for such a treatment is not fully met for our experimental conditions ($\gamma_{2B} \sim \gamma_{sp}$). A more complete analysis including both dephasing and losses from first principles is beyond the scope of this work, and of the theory developed in [18]. We determined the two-body loss rate $\gamma_{2B}$ directly from the experimental data, minimizing the $\chi^2$ between the model predictions and the measured atom number. Here $\gamma_{2B}$ is the only free parameter, and its best-fit value for each HL depth $V_\perp$ is shown in Fig. S3B. This fitted value of $\gamma_{2B}$ is chosen to plot all dashed curves in Figs. S4 and S5.

Note that this mean-field treatment does not accurately describe the dynamics at long times (see Fig. S5). The behavior captured empirically by Eq. (S33) could be a hint of many-body correlations building up dynamically in the system.

## VI. ANALYSIS OF THE MOMENTUM DISTRIBUTIONS

The main observable in our experiments is the measured atomic distribution after a time-of-flight expansion of $t_{\mathrm{tof}} = 20\,\mathrm{ms}$. In this section, we give the relevant details of the direct analysis (Figs. 1 and 2 of the main text) and of the fitting model (Figs. 3 and 4 of the main text).

### A. Direct analysis

*a. Peak amplitude* In Figs. 1 and 2 of the main article, we show the time evolution of the central $\boldsymbol{k} = 0$ peak amplitude of the measured momentum distributions for varying lattice depths $V_\perp$. Generally, the evolution of the peak amplitude shows a dramatic change between a fast decay for early times and an algebraic decay for longer times. For each $V_\perp$, we perform a fit using the phenomenological function presented in the Methods:

$$n_{\mathrm{peak}} = \frac{A}{(1+\gamma_{\mathrm{i}} t/\kappa)^{\kappa}}, \tag{S42}$$

which interpolates between the two behaviors. We show the best-fit parameters in Fig. S6. The starting time of the algebraic regime is related to the disappearance of long-ranged spatial coherence and narrow peaks in the momentum distribution, as discussed further in Sec. VI C.

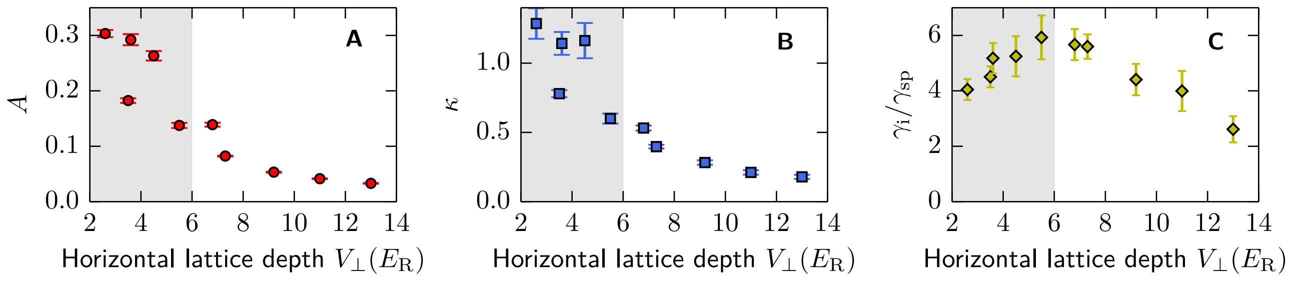


FIG. S6. **Best-fit parameters on $n(\boldsymbol{k}=0,t)$.** (**A** to **C**) Best-fit parameters using Eq. (S42) versus HL depth. $A$ is the initial central peak amplitude in the momentum distribution, $\kappa$ is the exponent characterizing its long-time algebraic decay and $\gamma_{\rm i}$ is its initial decay rate. Error bars are 1-sigma confidence intervals derived from a $\chi^2$ fitting procedure. The shaded areas show the region where the BH model is not a valid description.

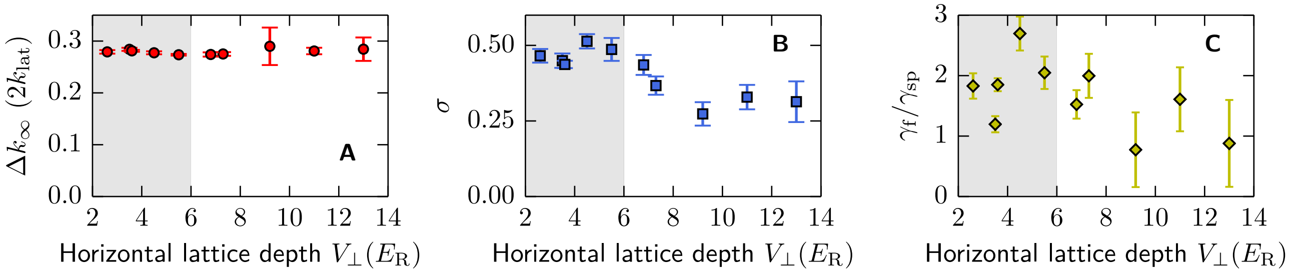


FIG. S7. **Best-fit parameters on $\Delta k$.** (**A** to **C**) Best-fit parameters using Eq. (S43) versus HL depth. $\Delta k_\infty$ is the final root-mean-square size, $\sigma$ is the exponent characterizing its short-time algebraic growth and $\gamma_{\rm f}$ is its rate. Error bars are 1-sigma confidence intervals derived from a $\chi^2$ fitting procedure. The shaded areas show the region where the BH model is not a valid description.

*b. Momentum width* In Fig. 1 of the main article, we show the time evolution of the root-mean-square (RMS) size of the momentum distribution $\Delta k_t = \int_{\rm BZ_1} k_x^2 n(\boldsymbol{k},t){\rm d}^2k$, where the integration is restricted to the first Brillouin zone BZ$_1$. This restriction is set in order to focus on the fundamental band dynamics, as well as including only the central Bragg peak. The observed saturation at long times is consistent with a uniform BZ$_1$ of width $2k_{\rm lat}$ and RMS size $k_{\rm lat}/\sqrt{3} \approx 0.29 \times 2k_{\rm lat}$. Generalizing Eq. (S9), we use the following form to fit the growth of momentum width $\Delta k = \sqrt{\Delta k_t^2 - \Delta k_{t=0}^2}$:

$$\Delta k = \sqrt{(\Delta k_\infty^2 - \Delta k_{t=0}^2)(1 - {\rm e}^{-(\gamma_{\rm f} t)^{2\sigma}})}. \tag{S43}$$

Here $\Delta k_\infty$ is the asymptotic size for long times, $\sigma$ the exponent characterizing the short-time power-law expansion and $\gamma_{\rm f}$ a rate related to the amplitude of the power-law. We show the best-fit parameters in Fig. S7. At short times, Eq. (S43) reduces to $\propto t^\sigma$, and the case of normal diffusion is $\sigma = 1/2$. In Fig. 1D, we only show the short-time $t^\sigma$ behavior inferred from such a fit. Note that the algebraic behavior of $\Delta k$ is similar to the algebraic behavior of $C_{\rm nn}$ (Fig. 1D and 4 of the main text). However, inter-band transitions and the initial structure factor of the gas makes this link non-trivial. In other words, there is no simple connection between the phenomenological Eq. (S43) and Eq. (S46).

## B. Extraction of coherence from the momentum profiles

### 1. *Momentum distribution and time of flight*

Under the assumption that interactions and finite time-of-flight effects can be neglected [32, 33], the time-of-flight distribution mirrors the initial momentum distribution $n(\boldsymbol{k})$ evaluated for $\boldsymbol{k} = M\boldsymbol{r}/(\hbar t_{\rm tof})$, with $\boldsymbol{r}$ the observation point. Using the basis of Wannier functions $w_{\boldsymbol{\nu}}(\boldsymbol{r} - \boldsymbol{r}_i)$, the normalized momentum distribution is given without further approximation by

$$n(\boldsymbol{k}) = \sum_{\text{bands}\,\boldsymbol{\nu}} \mathcal{S}_{\boldsymbol{\nu}}(\boldsymbol{k}) \mathcal{W}_{\boldsymbol{\nu}}(\boldsymbol{k}). \tag{S44}$$

Here, $\mathcal{W}_{\boldsymbol{\nu}}(\boldsymbol{k}) = |\widetilde{w}_{\boldsymbol{\nu}}(\boldsymbol{k})|^2$ is a smooth envelope function with $\widetilde{w}_{\boldsymbol{\nu}}$ the Fourier transform of $w_{\boldsymbol{\nu}}$, and $\mathcal{S}_{\boldsymbol{\nu}}$ is a normalized structure factor for band $\boldsymbol{\nu}$,

$$\mathcal{S}_{\boldsymbol{\nu}}(\boldsymbol{k}) = \frac{1}{N} \sum_{i,j} {\rm e}^{{\rm i}\boldsymbol{k}\cdot(\boldsymbol{r}_i - \boldsymbol{r}_j)} \langle \hat{a}^\dagger_{\boldsymbol{\nu},i} \hat{a}_{\boldsymbol{\nu},j} \rangle, \tag{S45}$$

*i.e.* a discrete Fourier transform of the correlation function $\langle \hat{a}^\dagger_{\boldsymbol{\nu},i} \hat{a}_{\boldsymbol{\nu},j} \rangle$.

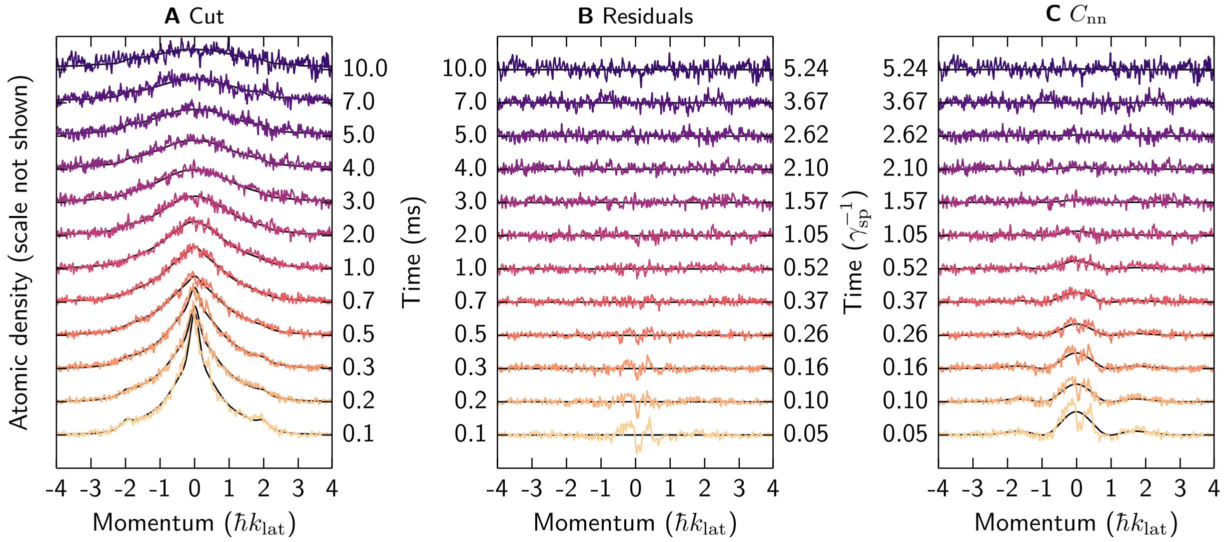


FIG. S8. **Fitting the momentum profiles.** (**A**) Momentum profiles $n(k_x, k_y = 0)$ along the $x$ axis of the optical lattice for several dissipation times increasing from bottom to top. The profiles correspond to times in the algebraic regime $t \geq \kappa/\gamma_{\rm i}$, and in-plane lattice depth $V_\perp = 7.3\,E_{\rm R}$. The solid lines show a fit to the model in Eq. (S47). (**B**) Residuals of the fit. (**C**) $C_{\rm nn}$ contribution in the fits, where we show the residual modulation provided by the part involving $C_{\rm nn}$. The profiles are averages over 3 realizations of the experiment.

### 2. *Fitting model*

The parametrization of the momentum distribution in Eq. (S44) is very general, but also too complicated to be of practical use. We truncate the sum in Eq. (S44) to make a fit to the experimental data tractable, and argue why this truncation is justified in the algebraic regime which is the focus of the article.

*a. Systems with short-range coherence* We first consider a system characterized by short-range coherence. The spatial correlation functions $\langle \hat{a}^\dagger_{\boldsymbol{\nu},i}\hat{a}_{\boldsymbol{\nu},j}\rangle$ fall off quickly with the separation $\boldsymbol{R} = \boldsymbol{r}_i - \boldsymbol{r}_j$, in such a way that the physical properties are well captured by the first two dominant terms with $\boldsymbol{R} = 0$ and $\boldsymbol{R} = \pm\boldsymbol{e}_{x/y}$, where $\boldsymbol{e}_{x/y}$ are the basis vector of the square lattice corresponding to nearest-neighbors. This regime corresponds in particular to the algebraic regime of the decay of spatial coherences that we report in the main text, and corresponds to a structure factor in the fundamental band

$$\mathcal{S}_0(\boldsymbol{k}) \approx P_0 + \sum_{\boldsymbol{R}=\pm\boldsymbol{e}_{x/y}} C_{\rm nn}\cos\left(\boldsymbol{k}\cdot\boldsymbol{R}\right). \tag{S46}$$

Although atoms initially populate only the fundamental band, we expect that inter-band transitions gradually populate the lowest excited bands. Since this inter-band transfer is driven by incoherent spontaneous processes, it is reasonable to neglect coherence in these excited bands, corresponding to structure factors in the excited bands $\mathcal{S}_{\boldsymbol{\nu}\neq 0}(\boldsymbol{k}) = P_{\boldsymbol{\nu}}$. Here $P_{\boldsymbol{\nu}} = 1/N\sum_i\langle \hat{a}^\dagger_{\boldsymbol{\nu},i}\hat{a}_{\boldsymbol{\nu},i}\rangle$ is the normalized population of the band $\boldsymbol{\nu}$.

These assumptions result in the following model for the momentum distribution of a system with short-range coherence,

$$n(\boldsymbol{k}) \approx \mathcal{S}_0(\boldsymbol{k})\mathcal{W}_{\boldsymbol{0}}(\boldsymbol{k}) + \sum_{\nu=1,\cdots,3} P_{\boldsymbol{\nu}}\mathcal{W}_{\boldsymbol{\nu}}(\boldsymbol{k}), \tag{S47}$$

where the free parameters are the populations $P_{\boldsymbol{\nu}}$ and the nearest-neighbor coherence $C_{\rm nn}$ in the fundamental band. The Wannier envelopes are calculated from the band structure [8] using the experimentally determined lattice depths.

*b. Non-zero condensed fraction* The preceding discussion assumes explicitly that there is no condensate with long-range phase coherence. Initially, a condensate is generally present (except for lattice depths high enough that the whole system is in the Mott insulator regime). In a broken-symmetry approach [34], the presence of a condensate translates in a non-vanishing expectation value of the bosonic field $\alpha_{\boldsymbol{r}_i} = \langle \hat{a}_{\boldsymbol{\nu}=\boldsymbol{0},i}\rangle \neq 0$. We account for a non-zero condensed fraction by assuming that the structure factor of the fundamental band can be written as the sum of a "coherent" component and of a short-ranged one,

$$\mathcal{S}_0'(\boldsymbol{k}) = \mathcal{S}_{0,\rm BEC}(\boldsymbol{k}) + \mathcal{S}_0(\boldsymbol{k}). \tag{S48}$$

The coherent component $\mathcal{S}_{0,\rm BEC}(\boldsymbol{k})$ describes the condensate as in the standard Gross-Pitaevskii theory [32]. For simplicity, we model it as the sum of Gaussian functions at the main reciprocal lattice vectors

$$\mathcal{S}_{0,\rm BEC}(\boldsymbol{k}) = A_0 G_{\rm BEC}(\boldsymbol{k}) + A_1 \sum_{\boldsymbol{K}=\pm 2k_{\rm lat}\boldsymbol{e}_{x/y}} G_{\rm BEC}(\boldsymbol{k}-\boldsymbol{K}). \tag{S49}$$

The first term corresponds to the central Bragg spot centered in the first Brillouin zone (BZ), of amplitude

$A_0$, and the other terms to the lateral spots centered in all copies of the second BZ, of amplitude $A_1$. The function $G_{\rm BEC}(\boldsymbol{k})$ is a normalized Gaussian function of fixed width. We calculate the width accounting for near field effects [33]. Using the expressions given in [33] and assuming a Thomas-Fermi profile, we obtain a near-Gaussian distribution of root-mean-square width $\sigma_{\rm BEC} \approx 0.13 \times k_{\rm lat}$ for the expansion time of 20 ms used in our experiments. The short-ranged component $\mathcal{S}_0(\boldsymbol{k})$ is treated as discussed before in Eq. (S46).

*c. Fit results* We fit Eq. (S47) in combination with Eq. (S48) to the measured momentum profiles. The free parameters are the amplitudes of the condensate peaks $A_0, A_1$ in Eq. (S49), the populations $P_{\boldsymbol{\nu}}$ and the nearest-neighbor coherence $C_{\rm nn}$ in Eq. (S47). We minimize the reduced $\chi^2 = (1/N_{\rm dof}) \times \int {\rm d}^2\boldsymbol{k}[n_{\rm obs}(\boldsymbol{k}) - n_{\rm fit}(\boldsymbol{k})]^2/\sigma^2_{\rm obs}$, with $n_{\rm obs}$ the observed distribution, $n_{\rm fit}$ the fitting model in Eq. (S48), $\sigma_{\rm obs}$ the typical noise on the images and $N_{\rm dof}$ the number of degrees of freedom, *i.e.* the number of data points minus the number of fit parameters.

Fig. S8 shows cuts through the 2D profiles along one lattice axis for $V_\perp = 7.3\,E_{\rm R}$, together with the fits (solid lines), residuals of the fits and $C_{\rm nn}$ contribution in the fits. The duration of the dissipation laser pulse increases from bottom to top. We find a good agreement between the observed profiles and the data. The residuals are comparable or lower than the imaging noise (corresponding to optical densities $\sim 0.02$ and dominated by photonic shot noise and residual imperfections of the fringe reduction algorithm). The reduced $\chi^2$ is roughly equal to 1 for all dissipation times. The $C_{\rm nn}$ contribution in the fits corresponds to the quantity $(\mathcal{S}_0(\boldsymbol{k}) - P_0)\mathcal{W}_{\boldsymbol{0}}(\boldsymbol{k})$. We tried to include second nearest-neighbor coherences in the fundamental band, or coherences in the excited bands. We found that it does not improve the quality of the fits. We also attempted to force coherence in the first excited band instead of the ground band, and systematically found a markedly higher $\chi^2$ value.

Because of a finite noise in the images (coming mostly from photon shot noise), the resolution in the determination of $C_{\rm nn}$ is also finite, and we estimate it around 0.01 to 0.02. Such a limitation explains the apparent long-times saturation of the signal for the highest lattice depth $V_\perp \geq 9\,E_{\rm R}$.

In order to complete the data presented in the main text, we show in Figs. S4 and S5 a full panel of the best-fit parameters evolution $C_{\rm nn}$ and $N$, along with the prediction from our model presented in Sec. V.

#### 3. Power-law fit

The emergent algebraic regime in the decay of the nearest-neighbor correlator $C_{\rm nn}$ only shows up in a "scaling" window. In order to extract a reliable power-law exponent from the evolution of $C_{\rm nn}$, we perform a power-law fit in a specific time window. The start of this window is chosen to be equal to $\kappa/\gamma_{\rm i}$, i.e. the start of the algebraic decay in the peak amplitude of the momentum distribution as explained in Sec. VI A. The end of the window is chosen at $2\,\gamma_{\rm sp}^{-1}$ in order to exclude data points that are either departing from the algebraic decay (for small $V_\perp$) or limited by detection (for high $V_\perp$).

### C. Evolution of condensed fraction

At the start of the algebraic regime for $t \gtrsim \kappa/\gamma_{\rm i}$, the condensed fraction is almost zero, and its contribution vanishes quickly. We are interested here in how it decays for earlier times. We first note from Fig. S6C that the initial decay rate $\gamma_{\rm i}$ is substantially higher than $\gamma_{\rm sp}$. Second, as shown in Fig. S9A, with the example value of $V_\perp \approx 7.3\,E_{\rm R}$, the diffraction peaks in the momentum distribution decay exponentially. We fit a decay rate $\gamma_{\rm BEC}$ from such a decay and compare it to the initial decay rate $\gamma_{\rm i}$ determined from the phenomenological analysis in Eq. (S42) and shown in Fig. S9B. The two analyses give decay rates in very good agreement. This suggests that our interpretation that the initial decay of the coherence is dominated by the loss of long-ranged coherence, captured by a condensed fraction in the cloud, is correct. The results are only shown for $V_\perp \leq 8\,E_{\rm R}$, for which the initial state is a superfluid. Above this limit the initial condensed fraction is small and barely discernible from noise. This arises from the vicinity of the Mott transition where strong interactions deplete the condensate.

Interestingly, we observe that the trend is similar to the evolution of the interaction strength (solid black line in Fig. S9B), which indicates a probable role played by the interactions in the initial decay of the coherence. A similar enhancement of the decay rate compared to non-interacting systems was also observed in the numerical calculations presented in [12].

### D. Inter-band transitions

We show in Fig. S10A the relative populations $P_{\boldsymbol{\nu}}$ of the fundamental and excited bands for a lattice depth $V_\perp \approx 7.3\,E_{\rm R}$. Similar curves are observed for other lattice depths. We observe that a substantial level of inter-band transitions occurs after a few milliseconds (corresponding to a few $\gamma_{\rm sp}^{-1}$, much longer than the initial decay time of the coherence). We show the initial rate of departure from the fundamental band ($\Gamma^0$) and the initial feeding rate of the first excited energy level ($\Gamma^1$) in Fig. S10B and C. The rates are roughly smaller than $\gamma_{\rm sp}$ and decrease with the lattice depth. This is consistent with the expectation of a transfer rate given by the product of the spontaneous emission rate and a matrix element describing the motional overlap between the initial and final states. The latter should be on the order of one or smaller and decrease with lattice depth.

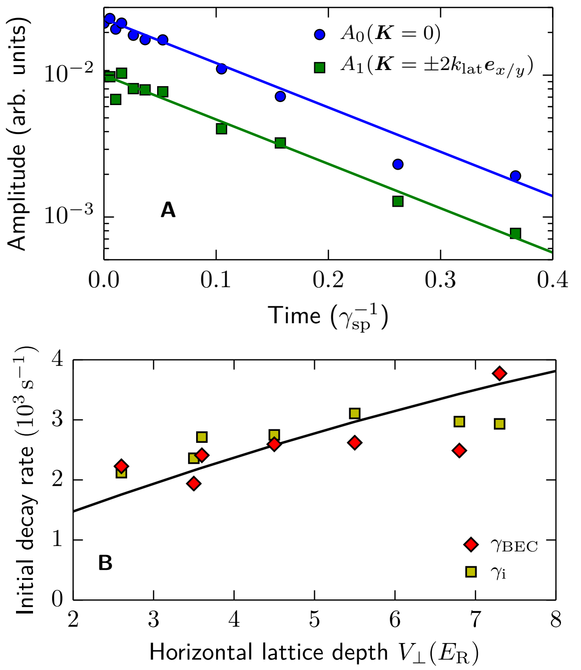


FIG. S9. **Initial coherence decay rates.** (**A**) Decay of the fitted condensed fraction peak amplitudes $A_0$ and $A_1$ [see Eq. (S49)]. The in-plane lattice depth is $V_\perp \approx 7.3\,E_{\mathrm{R}}$. The solid lines are exponential fits of $A_0$ and $A_1$ with an identical rate $\gamma_{\mathrm{BEC}} \approx 7.1\,\gamma_{\mathrm{sp}}$. (**B**) Comparison between both determinations of the initial decay rates: $\gamma_{\mathrm{i}}$ extracted from Eq. (S42) and $\gamma_{\mathrm{BEC}}$ extracted from fits as shown in (A). For comparison, we also show the quantity $0.85\,U/\hbar$ as a solid line.

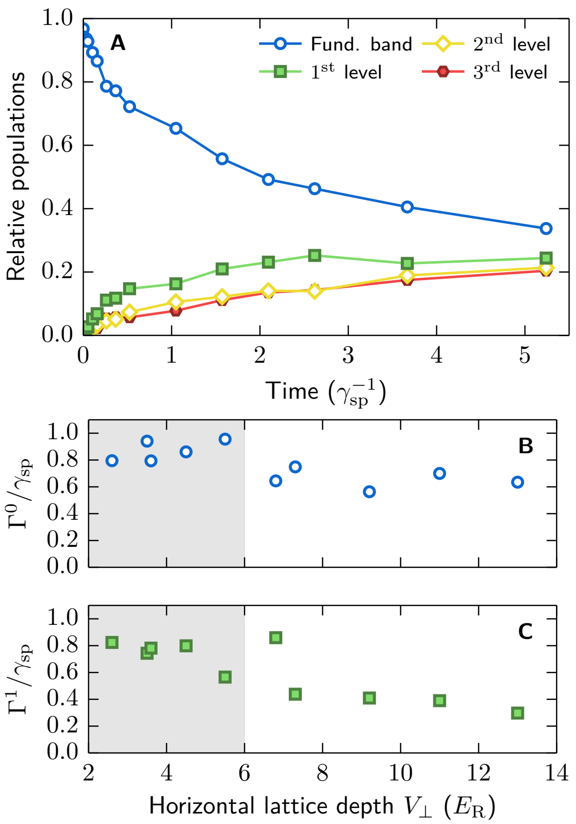


FIG. S10. **Observation of inter-band transitions.** (**A**) Relative populations in the fundamental and excited levels as a function of time for $V_\perp = 7.3\,E_{\mathrm{R}}$. (**B**) Initial rate of departure from the fundamental band $\Gamma^0$ taken as the slope of curves in (A) at early times. (**C**) Initial rate of feeding in the first excited energy level $\Gamma^1$. The same description as in (B) applies. The shaded areas show the region where the BH model is not a valid description.

[1] J. H. Denschlag, J. E. Simsarian, H. Häffner, C. McKenzie, A. Browaeys, D. Cho, K. Helmerson, S. L. Rolston, and W. D. Phillips, Journal of Physics B: Atomic, Molecular and Optical Physics **35**, 3095 (2002).

[2] R. Bouganne, M. Bosch Aguilera, A. Dareau, E. Soave, J. Beugnon, and F. Gerbier, New Journal of Physics **19**, 113006 (2017).

[3] W. Ketterle, D. S. Durfee, and D. M. Stamper-kurn, in *Proceedings of the International School of Physics Enrico Fermi*, Vol. 140, edited by M. Inguscio, S. Stringari, and C. Wieman (1999) pp. 67–176.

[4] C. Ockeloen-Korppi, A. Tauschinsky, R. Spreeuw, and S. Whitlock, Physical Review A **82**, 061606 (2010).

[5] D. S. Rokhsar and B. G. Kotliar, Physical Review B **44**, 10328 (1991).

[6] W. Krauth, M. Caffarel, and J.-P. Bouchaud, Physical Review B **45**, 3137 (1992).

[7] W. Zwerger, J. Opt. B: Quantum Semiclass. Opt. **5**, S9 (2003).

[8] I. Bloch, J. Dalibard, and W. Zwerger, Reviews of Modern Physics **80**, 885 (2008).

[9] J. Dalibard and C. Cohen-Tannoudji, Journal of Physics B: Atomic and Molecular Physics **18**, 1661 (1985).

[10] C. Cohen-Tannoudji, G. Grynberg, and J. Dupont-Roc, *Atom Photon Interactions*, Atomic and Molecular Physics (John Wiley & Sons, 1992).

[11] K. Ellinger, J. Cooper, and P. Zoller, Physical Review A **49**, 3909 (1994).

[12] H. Pichler, A. J. Daley, and P. Zoller, Physical Review A **82**, 063605 (2010).

[13] S. Haroche and J.-M. Raimond, *Exploring the Quantum: Atoms, Cavities, and Photons*, Oxford Graduate Texts (Oxford University Press, 2006).

[14] P. Marte, R. Dum, R. Taïeb, and P. Zoller, Physical Review A **47**, 1378 (1993).

[15] Y. Yanay and E. J. Mueller, Phys. Rev. A **90**, 023611 (2014).

[16] A. J. Daley, Advances in Physics **63**, 77 (2014), https://doi.org/10.1080/00018732.2014.933502.

[17] D. Poletti, J.-S. Bernier, A. Georges, and C. Kollath, Physical Review Letters **109**, 045302 (2012).

[18] D. Poletti, P. Barmettler, A. Georges, and C. Kollath, Physical Review Letters **111**, 195301 (2013).

[19] J. Weiner, V. S. Bagnato, S. Zilio, and P. S. Julienne, Rev. Mod. Phys. **71**, 1 (1999).

[20] M. T. DePue, C. McCormick, S. L. Winoto, S. Oliver, and D. S. Weiss, Physical Review Letters **82**, 2262 (1999).

[21] N. Schlosser, G. Reymond, I. Protsenko, and P. Grangier, Nature **411**, 1024 (2001).

[22] N. S. Kampel, A. Griesmaier, M. P. H. Steenstrup, F. Kaminski, E. S. Polzik, and J. H. Müller, Phys. Rev. Lett. **108**, 090401 (2012).

[23] W. S. Bakr, A. Peng, M. E. Tai, R. Ma, J. Simon, J. I. Gillen, S. Fölling, L. Pollet, and M. Greiner, Science **329**, 547 (2010).

[24] J. F. Sherson, C. Weitenberg, M. Endres, M. Cheneau, I. Bloch, and S. Kuhr, Nature **467**, 68 (2010).

[25] N. Syassen, D. M. Bauer, M. Lettner, T. Volz, D. Dietze, J. J. García-Ripoll, J. I. Cirac, G. Rempe, and S. Dürr, Science **320**, 1329 (2008).

[26] S. Tojo, M. Kitagawa, K. Enomoto, Y. Kato, Y. Takasu, M. Kumakura, and Y. Takahashi, Physical Review Letters **96**, 153201 (2006).

[27] M.-S. Kim, J. Lee, J. H. Lee, Y. Shin, and J. Mun, Physical Review A **94**, 042703 (2016).

[28] S. G. Porsev, M. S. Safronova, A. Derevianko, and C. W. Clark, Phys. Rev. A **89**, 012711 (2014).

[29] M. Borkowski, R. Ciuryło, P. S. Julienne, S. Tojo, K. Enomoto, and Y. Takahashi, Phys. Rev. A **80**, 012715 (2009).

[30] K. Burnett, P. S. Julienne, and K.-A. Suominen, Phys. Rev. Lett. **77**, 1416 (1996).

[31] F. Dalfovo, S. Giorgini, L. P. Pitaevskii, and S. Stringari, Reviews of Modern Physics **71**, 463 (1999).

[32] P. Pedri, L. Pitaevskii, S. Stringari, C. Fort, S. Burger, F. S. Cataliotti, P. Maddaloni, F. Minardi, and M. Inguscio, Physical Review Letters **87** (2001), 10.1103/PhysRevLett.87.220401.

[33] F. Gerbier, S. Trotzky, S. Fölling, U. Schnorrberger, J. D. Thompson, A. Widera, I. Bloch, L. Pollet, M. Troyer, B. Capogrosso-Sansone, N. V. Prokof'ev, and B. V. Svistunov, Physical Review Letters **101**, 155303 (2008).

[34] L. Pitaevskii and S. Stringari, *Bose Einstein condensation* (Oxford University Press, Oxford, 2003).
